# Supplementary material for: VISLA Benchmark: Evaluating Embedding Sensitivity to Semantic and Lexical Alterations
Source: arXiv:2404.16365 source file (2024-04-25)
Supplement: Supplementary file 1 [file additional-metrics.tex]

\begin{table}
\centering

\begin{tabular}{l l l l lll}
 & \multicolumn{3}{c}{Generic VISLA} & \multicolumn{3}{c}{Spatial VISLA}\\
 Models& precision\_at\_2(Avg) & recall\_at\_2(Avg) & average\_precision (mAP)  & precision_at_2(Avg)& recall_at_2(Avg)&average_precision (mAP)\\
BLIP-ITM-COCO & 0.8638232271 & 0.8638232271 & 0.9253168893  & 0.8046875& 0.8046875&0.8938802083\\
XVLM-16M-COCO & 0.8170606372 & 0.8170606372 & 0.9025351148  & 0.75546875& 0.75546875&0.8747395833\\
XVLM-16M-Flickr & 0.8144912641 & 0.8144912641 & 0.8983384721  & 0.7515625& 0.7515625&0.86875\\
ViLT-ITR-COCO & 0.8098663926 & 0.8098663926 & 0.8942274752  & 0.75078125& 0.75078125&0.8716145833\\
FLAVA & 0.7970195272 & 0.7970195272 & 0.8896882494  & 0.7296875& 0.7296875&0.8567708333\\
XVLM-16M & 0.7939362795 & 0.7939362795 & 0.8922576225  & 0.7265625& 0.7265625&0.8580729167\\
ViT-bigG-14 & 0.7918807811 & 0.7918807811 & 0.8848920863  & 0.72578125& 0.72578125&0.8578125\\
roberta-ViT-B-32 & 0.7918807811 & 0.7918807811 & 0.8859198356  & 0.725& 0.725&0.8602864583\\
AltCLIP & 0.7857142857 & 0.7857142857 & 0.8789825283  & 0.7234375& 0.7234375&0.85546875\\
xlm-roberta-large-ViT-H-14 & 0.7836587873 & 0.7836587873 & 0.8739294279  & 0.71953125& 0.71953125&0.8475260417\\
ViT-g-14 & 0.7795477903 & 0.7795477903 & 0.8797533402  & 0.71328125& 0.71328125&0.8434895833\\
ViT-H-14 & 0.7769784173 & 0.7769784173 & 0.8722165125  & 0.7125& 0.7125&0.8522135417\\
SegCLIP & 0.7754367934 & 0.7754367934 & 0.8863480644  & 0.7109375& 0.7109375&0.8341145833\\
xlm-roberta-base-ViT-B-32 & 0.7702980473 & 0.7702980473 & 0.8689619733  & 0.70546875& 0.70546875&0.8342447917\\
xlarge:ViT-L-14 & 0.7682425488 & 0.7682425488 & 0.8687906817  & 0.70234375& 0.70234375&0.844140625\\
RN50 & 0.7677286742 & 0.7677286742 & 0.8758136348  & 0.70234375& 0.70234375&0.833203125\\
RN50x4 & 0.7646454265 & 0.7646454265 & 0.8696471394  & 0.7015625& 0.7015625&0.8384114583\\
NegCLIP & 0.7620760534 & 0.7620760534 & 0.8675059952  & 0.69921875& 0.69921875&0.8348958333\\
RN101 & 0.7610483042 & 0.7610483042 & 0.8705035971  & 0.69375& 0.69375&0.8397135417\\
ViT-B-32 & 0.7605344296 & 0.7605344296 & 0.8726447413  & 0.690625& 0.690625&0.83046875\\
BLIP2 & 0.7559095581 & 0.7559095581 & 0.8574854402  & 0.68984375& 0.68984375&0.8337239583\\
ALIGN & 0.7528263104 & 0.7528263104 & 0.8651935594  & 0.68828125& 0.68828125&0.828125\\
RN50x64 & 0.7512846865 & 0.7512846865 & 0.8693045564  & 0.6875& 0.6875&0.8266927083\\
ViT-L-14 & 0.7507708119 & 0.7507708119 & 0.8616820829  & 0.67578125& 0.67578125&0.8196614583\\
large:ViT-B-16 & 0.7492291881 & 0.7492291881 & 0.8583418979  & 0.67421875& 0.67421875&0.83359375\\
CLIP-SVLC & 0.7487153135 & 0.7487153135 & 0.8630524152  & 0.66953125& 0.66953125&0.821875\\
RN50x16 & 0.7476875642 & 0.7476875642 & 0.8639945187  & 0.66796875& 0.66796875&0.8111979167\\
ALIP & 0.7451181912 & 0.7451181912 & 0.8669921206  & 0.65703125& 0.65703125&0.8052083333\\
XVLM-4M & 0.7291880781 & 0.7291880781 & 0.8668208291  & 0.653125& 0.653125&0.79765625\\
CyCLIP & 0.6911613566 & 0.6911613566 & 0.8274237753  & 0.64375& 0.64375&0.830078125\\
BLIP-Caption-COCO & 0.6428571429 & 0.6428571429 & 0.7928228845  & 0.6265625& 0.6265625&0.7739583333\\
 Null Baseline& 0.5& 0.5& 0.5833& 0.5& 0.5&0.5833\\

\end{tabular}

\end{table}
